# Supplementary material for: Smith-Purcell radiation from time grating
Source: arXiv:2311.07381 source file (2023-11-13)
Supplement: Supplementary file 1 [file supple_backup.tex]

%%%%%%%%%%%%%%%%%%%%%%%%%%%Supporting Info by Chas%%%%%%%%%%%%%%%%%%%%%%%%%%
\documentclass[11pt,a4paper]{article}
\usepackage[margin=1in]{geometry}
\usepackage[sort&compress,square,numbers]{natbib}
\usepackage{lipsum,times,graphicx,hyperref,cleveref}
\usepackage[labelfont=bf]{caption}
\usepackage{xcolor}

\title{\vspace{-2cm} {\large Supplementary Materials for}\\[-2mm] 
\textbf{Exceptional points unveiling the upper limit of fluorescence rates in non-Hermitian plexcitonic single-photon sources}
}
	
\author{Wenjie Zhou, Jingfeng Liu, Juanfeng Zhu, Dmitrii Gromyko, Lin Wu$^\ast$ and Chengwei Qiu$^\ast$\\ 
\small $^\star$Email: lin\_wu@sutd.edu.sg, chengwei.qiu@nus.edu.sg
}

\date{}

%\renewcommand{\figurename}{Fig.}
\renewcommand{\baselinestretch}{1.33} 
\renewcommand{\thepage}{S\arabic{page}}
\renewcommand{\thetable}{S\arabic{table}}
\renewcommand{\thefigure}{S\arabic{figure}}
\renewcommand{\theequation}{S\arabic{equation}}
%==============================Content=========================
\begin{document}\maketitle

% \section*{content}

% \textcolor{blue}{1.NCoM and parameters: (1)Fitting method; (2)Geometries with different gap thickness; $\kappa,g,\eta$ VS gap (3)4 more linear fitting VS 2XImE;
% 2.Emission field operator;
% 3.Fluorescence rates VS ratio for three dipole moments and their eigenfrequencies; 
% 4.Fluorescence rates VS gap thickness for three dipole moments, giving the geometry at EP;
% 5.Solving the problem with the equations of motion;}

\section*{SI-1. The field quantization model}

\begin{figure}[h]
\centering	
\includegraphics{figS1.pdf}
\caption{Fitting to quantize the LSP mode $\alpha$  at the gap thickness $d=3$ nm. The purple circles denote simulation results obtained from the Comsol RF module, and the black line illustrates the quantization fitting.
\label{fig:sup1}}
\end{figure}

In this section, we provide an overview of the method used to determine the coupling rate $g_\alpha$ and the decay rate $\kappa_\alpha$ of the LSP mode $\alpha$ through the numerical simulations. We simulate the behavior of an excited QE at the center of the gap volume by introducing a dipole source oscillating along the $z$-axis. The excited electric field can be described by solving the Helmholtz equation \cite{novotny2012principles} for the system with the QE placed at position $r_0$, which is written as below:
\begin{equation}
    E_{\rm{ex}}(r,\omega) = \frac{k^2}{\epsilon_0} {\rm{Im}}G(r,r_0,\omega)\cdot \vec{\mu}(\omega),
\label{eq:sup1}
\end{equation}
In this equation, ${\rm Im}G$ represents the imaginary part of the dyadic Green's function, and $k=\omega/c$ is the wave vector, where $\omega$ is the angular frequency and $c$ is the speed of light. The dipole moment of the point source is denoted by $\vec{\mu}(\omega)=\mu(\omega)\cdot\vec{e_z}$, where $\vec{e_z}$ is a unit vector along the $z$-direction. Since the electric fields in the $x$ and $y$ directions can be neglected in the gap, the excited field $E_{\rm ex}$ is primarily contributed by the imaginary part of $E_z$ \cite{scheel2009macroscopic}. By setting the source dipole moment as $\mu(\omega)=\epsilon_0/k^2$, we can calculate ${\rm{Im}}G_z(r_0,r_0,\omega)$ using the following equation:
\begin{equation}
    E_{\rm ex}(r_0,\omega)=\rm{Im}E_z (r_0,\omega)={\rm{Im}}G_z(r_0,r_0,\omega).
    \label{eq:sup2}
\end{equation}
The local density of states (LDOS) in the gap is defined as:  
\begin{equation}
    \rm{LDOS} (r_0,\omega)=\frac{6\omega}{\pi c^2}[\vec{e_z}\cdot{\rm{Im}}G_z(r_0,r_0,\omega)\cdot\vec{e_z}].
    \label{eq:sup3}
\end{equation}
Simultaneously, the excited electric field also serves as the electromagnetic environment for the quantum emitter (QE). The coupling strength between the QE and the localized excitation field $E_{\rm ex}$ is typically defined as the product of the dipole moment $\mu(\omega)$ and the LDOS \cite{medina2021few,saez2022plexcitonic}. Assuming a constant dipole moment $\mu(\omega) = \mu_e$, the localized coupling strength can be expressed as:
\begin{equation}
    \hbar g(\omega) = \mu_e\cdot\rm E_{\rm ex}=\mu_e^2\frac{\pi\omega}{6\epsilon_0}\rm{LDOS} (r_0,\omega).
    \label{eq:sup4}
\end{equation}
This coupling strength represents the interaction between the QE and the LSP mode $\alpha$ of the NCoM, and it plays a crucial role in the fluorescence dynamics and rate enhancement.  According to Ref. \cite{medina2021few}, the coupling strength can be fitted by the spectral density, which is a sum of Lorentzian peaks determined by the $g_i$ and $\kappa_i$ of the isolated LSP modes. The spectral density $J(\omega)$ is given by:
\begin{equation}
    J(\omega) = \sum_i \hbar g_i^2 \frac{\kappa_i/2}{(\omega_i-\omega)+\kappa_i/4}.
    \label{eq:sup5}
\end{equation}
For the isolated mode $\alpha$ in our study, we can achieve:
\begin{equation}
    J_\alpha(\omega) = \hbar g_\alpha^2 \frac{\kappa_\alpha/2}{(\omega_\alpha-\omega)+\kappa_\alpha/4}=\mu_e^2\frac{\pi\omega}{6\epsilon_0}\rm{LDOS} (r_0,\omega).
    \label{eq:sup6}
\end{equation}
The case study we consider is a silver nanocube with sharp corners, neglecting the practical effect of edge rounding \cite{grillet2011plasmon}. The material dielectric constants are taken from \cite{johnson1972optical}. The LDOS is calculated by Eq. (\ref{eq:sup3}) from the simulation results obtained from the Comsol RF module.
In Fig. \ref{fig:sup1}, we perform the fitting of $J_\alpha(\omega)$ to $\hbar g(\omega)$ with a fixed gap thickness $d=3$ nm.  By the fitting, we obtain $g_\alpha=29.4$ meV and $\kappa_\alpha=167.7$ meV from a dipole moment $\mu_e=30$ D.
We further observe that the coupling rate $g_\alpha$ is directly proportional to the dipole moment $\mu_e$ due to the relationship in Eq. (\ref{eq:sup6}), $i.e.$, in this case study, $g_\alpha=0.98\mu_e$. This implies that $g_\alpha$ can be engineered by adjusting $\mu_e$ without altering the NCoM geometry. 
The above method, based on the Lorentzian nature of the isolated lossy modes, has been widely used to quantize plasmonic cavities in the quasi-static approximation \cite{delga2014quantum,cuartero2018light,varguet2019non}. Note that our study considers the LSP modes as orthogonal to each other, neglecting the destructive interference between neighboring modes.

\section*{SI-2. Derivation of the fluorescence operator}

In this section, we revisit the derivation of the fluorescence operator using the input-output formalism. To account for the loss in the system, we employ the Heisenberg-Langevin approach, which treats the dissipation as coupling with the reservoir modes \cite{waks2010cavity}. We introduce two additional terms to the system Hamiltonian, representing the reservoir and its interaction with the QE-LSP system. These terms can be expressed as follows:
\begin{eqnarray}
\hat{H}_{\rm res} = \int\hbar(\omega-\omega_{\rm L})\left[\hat{\rm b}^{\dagger}(\omega)\hat{\rm b}(\omega) + \hat{\rm c}^{\dagger}(\omega)\hat{\rm c}(\omega) \right]d\omega\;,
\\
\hat{H}_{\rm loss} = \int\sum_i \hbar\left[B_i\hat{\rm b}^{\dagger}(\omega)\hat{a}_i + F_i\hat{\rm c}^{\dagger}(\omega)\hat{a}_i\right]d\omega + \int \hbar F_e\hat{\rm c}^{\dagger}(\omega)\hat{\sigma}d\omega + \rm{H.c.}.
\end{eqnarray}
Here, $\hat{\rm b}^{\dagger}(\omega)$ and $\hat{\rm c}^{\dagger}(\omega)$ are the annihilation reservoir operators for the absorptive heat bath and the continuum radiative modes, respectively. They are coupled to the QE and LSP modes through the coupling rates $F_e$, $B_i$, and $F_i$.
For the simplified QE-LSP system with a single LSP mode $\alpha$, the evolution of the reservoir operators can be deduced from the Heisenberg-Langevin equations of motion. They are described in the form of:
\begin{eqnarray}
\hat{\rm b}(\omega,t)=\hat{\rm b}(\omega,0)e^{i\omega t}+\int_0^t B_\alpha \hat{a}_\alpha e^{-i\omega(t-t^{'})}dt^{'}\;,
\label{eq:motion1}
\\
\hat{\rm c}(\omega,t)=\hat{\rm c}(\omega,0)e^{i\omega t}+\int_0^t (F_\alpha \hat{a}_\alpha+F_e\hat{\sigma})e^{-i\omega(t-t^{'})}dt^{'}\;,
\label{eq:motion2}
\end{eqnarray}
Using the input-output formalism \cite{walls2008input}, we can define the output field operator as:
\begin{equation}
    \hat{\rm X}_{\rm out}(t)=\frac{1}{\sqrt{2\pi}}\int_{-\infty}^{\infty}\hat{\rm X}_{\rm out}(\omega,\tau)e^{-i\omega(t-\tau)}d\omega,
\label{eq:output}
\end{equation}
where $\tau$ is the terminal time when the evolution ends. By plugging Eq. (\ref{eq:output}) into Eq. (\ref{eq:motion1}) and Eq. (\ref{eq:motion2}), we can obtain the radiative output operator:
\begin{equation}
    \hat{\rm c}_{\rm out}(t)=\frac{1}{\sqrt{2\pi}}\int_{-\infty}^{\infty}\hat{\rm c}(\omega,0)e^{-i\omega t}d\omega + \sqrt{2\pi}(F_\alpha \hat{a}_\alpha + F_e \hat{\sigma}),
\end{equation}
and the nonradiative operator:
\begin{equation}
    \hat{\rm b}_{\rm out}(t)=\frac{1}{\sqrt{2\pi}}\int_{-\infty}^{\infty}\hat{\rm b}(\omega,0)e^{-i\omega t}d\omega + \sqrt{2\pi}B_\alpha \hat{a}_\alpha.
\end{equation}
Since the initial condition of the output field is in the vacuum state, we can neglect the terms  $\hat{\rm c}(\omega,0)$ and $\hat{\rm b}(\omega,0)$. By comparing the coefficients in the equations of motion \cite{waks2010cavity}, we find the relations for the coupling rates $F_e$, $B_i$, and $F_i$ as $\gamma_0 = 2\pi F_e^2$, $\kappa_{\rm r}=2\pi F_\alpha^2$, and $\kappa_{\rm nr}=2\pi B_\alpha^2$, where $\gamma_0$ is the vacuum spontaneous decay rate of the QE and $\kappa_{\rm r}$, $\kappa_{\rm nr}$ are radiative and nonradiative decay rates of the mode $\alpha$. 
Then the radiative output operator follows:
\begin{equation}
    \hat{\rm c}_{\rm out}(t)= \sqrt{2\pi}(F_\alpha \hat{a}_\alpha + F_e \hat{\sigma}).
\end{equation}
As we introduce the quantum yield $\eta_\alpha = \kappa_{\rm r}/(\kappa_{\rm r} + \kappa_{\rm nr})$ and set the total decay rate $\kappa_\alpha = \kappa_{\rm r} + \kappa_{\rm nr}$, finally, we deduce the fluorescence operator as 
\begin{equation}
    \hat{F}=\hat{\rm c}_{\rm out}=\sqrt{\gamma_0}\hat{\sigma}+\sqrt{\eta_\alpha \kappa_\alpha}\hat{a}_\alpha.
\end{equation}

\section*{SI-3. Fluorescence rates deduced from the decomposition of the master equation}

This section reviews the analytic method to solve the fluorescence rates by decomposing the master equation.  As demonstrated through linear fitting in Fig. 2(a), we have successfully established a direct equivalence between the fluorescence rate and the QE decay rate, $i.e.$, $\gamma_{\rm F}=\gamma_e$. Thus, in order to determine the fluorescence rate, we need to solve for the QE decay rate.
Fluorescence emission involves the decay of an initially excited atom with
no photon in the LSP mode, which is started from the initial quantum state:
\begin{equation}
    |\psi(0)\rangle = |\rm{QE},1\rangle + |\rm{LSP}_\alpha,0\rangle.
\end{equation}
Since the loss of the excitation is irreversible, we use the one-quantum state \cite{meystre2007elements} to describe the resonance between the QE and the LSP mode $\alpha$ ($i.e.$, the detuning is ignored):
\begin{equation}
    |\psi(t)\rangle = C_e(t) |{\rm{QE}},1\rangle + C_\alpha(t) |\rm{LSP}_{\alpha},1\rangle.
\end{equation}
whose evolution is governed by the equations of motion:
\begin{eqnarray}
\dot{C_e}(t) = -\frac{\gamma_0}{2}{C_e}(t)-ig_\alpha C_\alpha(t)\;,
\\
\dot{C_\alpha}(t) = -\frac{\kappa_\alpha}{2}C_\alpha(t)-ig_\alpha {C_e}(t).
\end{eqnarray}
In the weak coupling regime defined as $g_\alpha\ll\kappa_\alpha$ \cite{meystre2007elements}, the subsequent approximation is derived as follows:
\begin{eqnarray}
{C_\alpha}(t) = -\frac{ig_\alpha}{\kappa_\alpha/2}{C_e}(t)\;,
\\
\dot{C_e}(t) = -\left( \frac{\gamma_0}{2}+\frac{g_\alpha^2}{\kappa_\alpha/2} \right){C_e}(t)\;.
\end{eqnarray}
Hence the exited state population of the QE decays exponentially with the rate
\begin{equation}
    \gamma_e = \gamma_0+\frac{4g_\alpha^2}{\kappa_\alpha}，
\end{equation}
which also serves as an approximation of Eq. (7) for $g_\alpha\ll\kappa_\alpha$ in the main text.

In the strong coupling regime, the system exhibits Rabi oscillations, resulting in the coefficient ${C_e}(t)$ taking the form of:
\begin{equation}
{C_e}(t) = C_{e1} e^{e_1 t}+C_{e2} e^{e_2 t},
\end{equation}
where
\begin{equation}
    e_{1,2}=\frac{1}{2}\left( \frac{\gamma_0}{2}+\frac{\kappa_\alpha}{2} \right)\pm \frac{1}{2}\left[\left(\frac{\gamma_0}{2}+\frac{\kappa_\alpha}{2}\right)^2-4g_\alpha^2\right]^2.
\end{equation}
The exponents are reduced to
\begin{equation}
    e_{1,2}=-\frac{1}{2}\left( \frac{\gamma_0}{2}+\frac{\kappa_\alpha}{2} \right)\pm ig_\alpha,
\end{equation}
due to the strong coupling condition $g_\alpha\gg\kappa_\alpha$ \cite{meystre2007elements}. Since the real components of $e_{1,2}$ represent the decay and the two terms have the same contribution to the decay, the QE decay rate is deduced as:
\begin{equation}
    \gamma_e=\frac{\kappa_\alpha+\gamma_0}{2},
\end{equation}
which also agrees with our conclusion in the main text.

\section*{SI-4. Additional cases of analytical solution versus dynamic calculations }
\begin{figure}[h]
\centering	
\includegraphics{figS4.pdf}
\caption{The circles represent the fluorescence rates obtained from linear fitting of the dynamics, with each color denoting a distinct gap thickness. The lines illustrate the corresponding values deduced from $\gamma_+=2|{\rm Im}E_+|$.
\label{fig:sup4}}
\end{figure}
We present three additional examples in Fig. \ref{eq:sup4}, akin to the scenario illustrated by Fig. 2(b) in the main text, to explore fluorescence rates across different geometries. These examples involve gap thicknesses of 1.0, 2.6, and 4.4 nm. Impressively, we observe a striking congruence between outcomes obtained through two distinct methodologies: linear fitting of dynamics computed via the master equation and the analytical method via solving the imaginary component of the eigenfrequency $E_+$. This strong consistency supports the notion that fluorescence rates can indeed be determined by the analytical solution $2|{\rm Im}E_+|$. The alignment between these two approaches bolsters our confidence in the method's accuracy and reliability in this study.

\section*{SI-5. The impact of overlapping bright and dark modes }

\begin{figure}[h]
\centering	
\includegraphics{figS5.pdf}
\caption{(a). Spectra of the normalized LDOS and QY for the NCoM, excited by a dipole source at the position of the QE. The NCoM geometry is altered by varying the gap thickness from 1.0 to 4.4 nm in 0.2 nm increments. (b). Normalized radiative power and nonradiative power, depicted by the solid and dotted pink lines, respectively, are measured for a specific $d=3.6$ nm. The grey curve portrays the corresponding QY, revealing its deviation from the resonant frequency.
\label{fig:sup2}}
\end{figure}

In this section, we delve into the implications of mode overlap between $\alpha$ and $\beta$ on the quantization of the bright mode $\alpha$. As depicted in Fig. \ref{fig:sup2}(a), our exploration centers on the QY as an indicator of the influence stemming from mode $\beta$. The QY is evaluated using the formula $\eta_\alpha = P_{\rm{r}}/(P_{\rm{r}}+P_{\rm{nr}})$ \cite{novotny2012principles}, extracted from simulations, with $P_{\rm r}$ and $P_{\rm nr}$ denoting the radiative and nonradiative power, respectively.

Analysis of the QY peaks uncovers deviations from the behavior of mode $\alpha$, exacerbated as the gap thickness increases and mode overlapping deteriorates. Furthermore, Fig. \ref{fig:sup2}(b) offers insight into the nonradiative and radiative power distribution at a specific gap thickness, $d=3.6\,{\rm nm}$. Evidently, overlapping regions between the modes lead to enhanced nonradiative power and suppressed radiative power, causing the QY to shift towards the left.

Although the subsequent fluorescence rate analysis does not factor in the QY, the overlapping of the two modes significantly impacts the accuracy of quantization fitting. This influence becomes particularly pronounced for gap thicknesses exceeding our designated range, complicating the differentiation of mode $\alpha$'s resonant frequency. In essence, we set a cap of 4.4 nm for the gap thickness to mitigate these challenges arising from mode overlap, ensuring precise and reliable quantization outcomes.

\section*{SI-6. Additional cases for the maximum fluorescence rates at EPs}

\begin{figure}[h]
\centering	
\includegraphics[scale=0.9]{figS6.pdf}
\caption{
Engineering the fluorescence rate based on the maximum values at the EPs. (a) and (b) depict the eigenfrequencies corresponding to the dipole moments $\mu_e=25$ D and $35$ D, respectively, as a function of normalized coupling rates. (c) and (d) display the corresponding fluorescence rates. (e) illustrates the fluorescence rates for three different dipole moments as a function of gap thickness.
\label{fig:sup4}}
\end{figure}

We have presented the eigenfrequencies and fluorescence rates obtained from the alternated dipole moments $\mu_e =25$ and $35$ D  in Fig. \ref{eq:sup4}. The results align closely with the observations made in the main text, reinforcing the notion that, at a consistent dipole moment, EPs correspond to complete coalescence states, yielding the highest fluorescence rate. In practical applications, optimizing fluorescence rates can be achieved by targeting EPs and optimizing system geometries accordingly. This straightforward optimization workflow based on EPs provides a promising approach for enhancing fluorescence rates.

Our exploration of the optimization workflow extends to examining dipole moments' influence. Illustrated in Fig. \ref{eq:sup4}(e), we present the fluorescence rates for dipole moments $\mu_e = 25$ D, $30$ D, and $35$ D, plotted against the gap thickness $d$. Drawing from the quantization method, it's established that the coupling rate $g_\alpha$ maintains proportionality with  $\mu_e$. Concurrently, the decay rate $\kappa_\alpha$ is distinctly governed by the gap thickness alone. Within the regime of strong coupling, these three curves harmoniously coincide. Here, fluorescence rates predominantly hinge on the gap thickness, denoted as $(\kappa_\alpha+\gamma_0)/2$, while shifts in coupling rates stem from variations in dipole moments during the weak coupling regime.

The highest fluorescence rates observed in Fig. \ref{eq:sup4}(e) are approximately 45.3 meV at $d\simeq$ 2.3 nm for $\mu_e=$ 25 D, 57.5 meV at $d\simeq$ 2.5 nm for $\mu_e=$ 30 D, and 60.6 meV at $d\simeq$ 2.6 nm for $\mu_e=$ 35 D. The enhancement of the highest rates, along with the corresponding optimal gap thickness at the EPs underscores the potential of achieving optimized fluorescence rates by utilizing larger dipole moments, which in turn reduces fabrication challenges. This observation explains the growing interest in studying the performance of quantum dots, molecules, and defects that can serve as quantum emitters, as larger dipole moments offer the potential for higher optimized rates.

Overall, our findings underscore the importance of considering dipole moments and gap thickness in optimizing fluorescence rates. By leveraging EPs and larger dipole moments, it is possible to overcome fabrication difficulties and attain higher optimized rates, providing valuable insights for future research and development in this field.


\section*{SI-7. Intuitive fluorescence rate analysis near EPs}

\begin{figure}[ht]
\centering
\includegraphics[scale=1]{figS7.pdf}
\caption{\label{fig:sup3}Each rainbow curve depicts the fluorescence rate variation with the dipole moment of the QE (expressed as the varying of $g_\alpha$) for each gap thickness. With increasing gap thickness, the EPs associated with each curve, denoted by the sharp turning corners on the curves, shift progressively to the right.  Notably, the fluorescence rates for specific dipole moments of 25 D, 30 D, and 35 D are indicated by green stars, magenta circles, and blue squares, respectively. All three maximum fluorescence rates consistently align with specific EPs. }
\end{figure}

The rainbow curves depicting the fluorescence rate variation with the dipole moment of the QE (expressed as the varying of $g_\alpha$) for each gap thickness are presented in Fig. \ref{fig:sup3}.

    The saturated fluorescence rates increase with increasing gap thickness $d$.  However, simultaneously, the EPs on the turning points of the saturation shift towards the right, demanding higher coupling rates to achieve strong coupling. In the weak coupling regime, the curves associated with smaller gaps are positioned higher compared to those of larger gaps. This implies that the points corresponding to specific dipole moments on the weak arms of the curves display an ascending pattern as the gap thickness decreases from 4.4 nm to 2.6 nm. In contrast, within the strong coupling regime, the points along the strong arms of the curves exhibit a declining trend as the gap thickness increases from 2.6 nm to 1.0 nm. When $g_\alpha$ varies monotonically with $d$ (as depicted in Fig. \ref{fig3}(b)), the opposites trends on the weak and strong arms of the curves inherently lead to a maximum fluorescence rate for a specific dipole moment situated precisely at the boundary between weak and strong coupling, namely, at the EP.

To illustrate this behavior, the three examples with the dipole moments of 25, 30 and 35 D are provided. These examples highlight their rapid and increasingly accelerated growth as they approach their respective EPs.

\bibliography{supple1}
\bibliographystyle{apalike}

\end{document}
